# Supplementary material for: Revisiting and Exploring Efficient Fast Adversarial Training via LAW: Lipschitz Regularization and Auto Weight Averaging
Source: arXiv:2308.11443 source file (2023-08-22)
Supplement: Supplementary file 1 [file appendix.tex]

This appendix contains the following contents:

\begin{itemize}
\item Summary of the existing FAT in Sec.~\ref{sec:summarize} of the manuscript.
(see Appendix~\ref{appendix:summarize}).

\item Detail description of the sample initialization used in the existing FAT in  Sec.~\ref{sec:Initialization} of the manuscript.
(see Appendix~\ref{appendix:initialization}).

\item More results of FGSM-BR with different data augmentation methods in Sec.~\ref{sec:Augmentation} of the manuscript
(see Appendix~\ref{appendix:augmentation}). 
 
\item Proof to the effectiveness of the
proposed regularization in Sec.~\ref{sec:regularization} of the manuscript.
(see Appendix~\ref{appendix:proof}). 

% \item Detailed algorithms of our FGSM-LAW in Sec.~\ref{sec:algorithm} of the manuscript.

% \item Description of these databases
% in Sec.~\ref{sec:algorithm} of the manuscript (see Sec.~\ref{appendix:databases}). 

\item Results of the comparative experiments with a cyclic learning rate strategy in Sec.~\ref{sec:cyclic} of the manuscript.
(see Appendix~\ref{appendix:cyclic}). 

\item Detailed hyper-parameter settings in Sec.~\ref{sec:cyclic} of the manuscript.
(see Appendix~\ref{appendix:hyper-parameter}).

\item Experiments with WideResNet34-10 as the backbone in Sec.~\ref{sec:wideresnet} of the manuscript.
(see Appendix~\ref{appendix:WideResNet}).

\item Experiments on Tiny ImageNet and ImageNet in Sec.~\ref{sec:ImageNet} of the manuscript.
(see Appendix~\ref{appendix:ImageNet}). 
% It can be observed that combined with Cutout, Mixup, CutMix and AutoAugment, FAT can achieve better robustness performance in all the attack scenarios. Particularly, under the PGD-10 attack, Cutout improves the performance by about 4.5\% without additional training cost.
\end{itemize}

\section{summary of the existing fast adversarial training methods}
\label{appendix:summarize}
We investigate the used techniques of more than tens of papers working on
the FAT methods. The summary is shown in Table~\ref{table:cifar10_implement}. It can be observed that different FAT methods require different training costs, \emph{i.e,} training time and memory costs.

\section{Detail description of the sample initialization used in the existing FAT}
\label{appendix:initialization}
\input{latex/appendix_init}

\begin{table*}[t]
\centering
\caption{ The techniques used in different fast adversarial training methods on CIFAR-10. 
% Number in bold indicates the best of the fast AT methods. 
}
\label{table:cifar10_implement}

\scalebox{0.82}{
\begin{tabular}{@{}c|c|c|c|c|c|c|c|c@{}}
\toprule
  Method        & Initialization & \begin{tabular}[c]{@{}c@{}}Step \\ Size\end{tabular} & Regularization & \begin{tabular}[c]{@{}c@{}}Training \\ Time\end{tabular} & \begin{tabular}[c]{@{}c@{}}Data \\ Memory \end{tabular} & \begin{tabular}[c]{@{}c@{}}Early \\ Stop\end{tabular} & \begin{tabular}[c]{@{}c@{}}CO w/o \\ Early Stop\end{tabular} & \begin{tabular}[c]{@{}c@{}}\textgreater 45\% \\ under AA\end{tabular} \\ \midrule \midrule
FGSM-AT   &      $\eta = 0 $       & $\epsilon$         & \usym{2717}             & 1 $\times$   &     \begin{tabular}[c]{@{}c@{}}One \\ Batch \end{tabular}       & \usym{2714}        & \usym{2714}               & \usym{2717}                         \\ \midrule
Free-AT   &        $\eta = 0 $        & $\epsilon$          & \usym{2717}             & 4.2 $\times$  &     \begin{tabular}[c]{@{}c@{}}One \\ Batch \end{tabular}        & \usym{2717}         & \usym{2717}                & \usym{2717}                         \\ \midrule
FGSM-RS   &     $\eta \in \mathbf{U}(-\epsilon, \epsilon)$           & 1.25$\epsilon$       & \usym{2717}             & 1 $\times$   &     \begin{tabular}[c]{@{}c@{}}One \\ Batch \end{tabular}          & \usym{2714}        & \usym{2714}               & \usym{2717}                         \\ \midrule
FGSM-GA   &     $\eta \in \mathbf{U}(-\epsilon, \epsilon)$           & 1.25$\epsilon$       & \usym{2714}            & 3.5 $\times$   &     \begin{tabular}[c]{@{}c@{}}One \\ Batch \end{tabular}         & \usym{2714}        & \usym{2717}                & \usym{2717}                         \\ \midrule
FGSM-CKPT &    $\eta \in \mathbf{U}(-\epsilon, \epsilon)$            & 1.25$\epsilon$    & \usym{2717}             & 1.5 $\times$   &     \begin{tabular}[c]{@{}c@{}}One \\ Batch \end{tabular}        & \usym{2717}         & \usym{2717}                & \usym{2717}                         \\ \midrule
ATTA      &    $\eta_{t+1}=\boldsymbol{\delta}_{E} $             & $\epsilon$          & \usym{2717}             & 1 $\times$    &     \begin{tabular}[c]{@{}c@{}}Whole \\ Dataset \end{tabular}         & \usym{2717}         & \usym{2717}                & \usym{2717}                         \\ \midrule
NuAT      &    $\eta \in \mathbf{B}(-\epsilon/2, \epsilon/2)$            & $\epsilon$          & \usym{2714}            & 2 $\times$     &     \begin{tabular}[c]{@{}c@{}}One \\ Batch \end{tabular}         & \usym{2717}         & \usym{2717}                & \usym{2714}                        \\ \midrule
GAT       &   $\eta \in \mathbf{B}(-\epsilon/2, \epsilon/2)$              & $\epsilon$          & \usym{2714}            & 2 $\times$  &     \begin{tabular}[c]{@{}c@{}}One \\ Batch \end{tabular}          & \usym{2717}         & \usym{2717}                & \usym{2714}                        \\ \midrule
SLAT      &      $\eta \in \mathbf{U}(-\epsilon, \epsilon)$          & $\epsilon$          & \usym{2714}            & 1.1 $\times$   &     \begin{tabular}[c]{@{}c@{}}One \\ Batch \end{tabular}         & \usym{2717}         & \usym{2717}                & \usym{2717}                         \\ \midrule
FGSM-SDI  &       $\eta=\epsilon \cdot g\left(,\theta\right)$         & $\epsilon$          & \usym{2717}             & 1.6 $\times$   &     \begin{tabular}[c]{@{}c@{}}One \\ Batch \end{tabular}        & \usym{2717}         & \usym{2717}                & \usym{2714}                        \\ \midrule
FGSM-PGI  &        $\eta_{t+1}=\boldsymbol{\delta}_{P} $       & $\epsilon$         & \usym{2714}            & 1.4 $\times$    &     \begin{tabular}[c]{@{}c@{}}Whole \\ Dataset \end{tabular}       & \usym{2717}         & \usym{2717}                & \usym{2714}                        \\ \bottomrule
\end{tabular}
}
\end{table*}
\input{table/augmentation}
\input{table/cifar10_cyclic}

\begin{table}[t]
\centering
\caption{ Test robustness (\%) on the CIFAR-10 database using WideResNet34-10 with different adversarial training methods. Number in bold indicates the best. 
% Number in bold indicates the best of the fast AT methods. 
}
\label{table:cifar10_wide}
\scalebox{0.92}{

\begin{tabular}{@{}c|c|c|c|c|c|c@{}}
\toprule
CIFAR-10  & Clean          & PGD-10         & PGD-20         & PGD-50         & AA             & Time \\ \midrule
PGD-AT    & 85.17          & 56.1           & 55.07          & 54.87          & 51.67          & 5.2 $\times$ \\ \midrule  \midrule
FGSM-RS   & 74.3           & 42.3           & 41.2           & 40.9           & 38.4           & 1 $\times$   \\ \midrule
FGSM-PGI  & 85.09          & 57.72          & 56.86          & 56.4           & 50.11          & 1.4 $\times$ \\ \midrule
FGSM-CKPT & \textbf{91.84} & 44.7           & 42.72          & 42.25          & 40.46          & 1.5 $\times$  \\ \midrule
FGSM-SDI  & 86.4           & 55.89          & 54.95          & 54.6           & 51.17          & 1.6 $\times$ \\ \midrule
NuAT      & 85.30          & 55.8           & 54.68          & 53.75          & 50.06          & 2.0 $\times$ \\ \midrule
GAT       & 85.17          & 56.3           & 55.23          & 54.97          & 50.01          & 2.0 $\times$  \\ \midrule
FGSM-GA   & 82.1           & 48.9           & 47.1           & 46.9           & 45.7           & 3.5 $\times$ \\ \midrule
Free-AT   & 80.1           & 47.9           & 46.7           & 46.3           & 43.9           & 4.2 $\times$ \\ \midrule
Ours      & 84.78          & \textbf{59.88} & \textbf{59.26} & \textbf{59.12} & \textbf{52.29} & 1.4 $\times$ \\ \bottomrule
\end{tabular}
}
\end{table}

\section{Proof to the effectiveness of the
proposed regularization}
\label{appendix:proof}

Actually the proposed regularization corresponds to a new sample-based local linearity metric of loss function $\ell$ corresponding to $(\mathbf{x},\mathbf{y})$ and $\boldsymbol{\delta}$:
\begin{equation}
\mathbb{E}_{\boldsymbol{\eta}}\left[\frac{\left|f(\mathbf{x}+\boldsymbol{\delta} ; \boldsymbol{\theta})-f(\mathbf{x}+\boldsymbol{\eta} ; \boldsymbol{\theta})\right|}{\|\boldsymbol{\delta}-\boldsymbol{\eta}\|_2}\textbf{}\right].
\end{equation}
This metric is bounded with the gradient of $f$ at $(\mathbf{x}+\boldsymbol{\delta},\mathbf{y})$ as
\begin{equation}
    \begin{aligned}
    & & &\ \ \mathbb{E}_{\boldsymbol{\eta}}\left[\frac{\left|f(\mathbf{x}+\boldsymbol{\delta} ; \boldsymbol{\theta})-f(\mathbf{x}+\boldsymbol{\eta} ; \boldsymbol{\theta})\right|}{\|\boldsymbol{\delta}-\boldsymbol{\eta}\|_2}\textbf{}\right]\\[3pt]
    & &\leq&\ \ \mathbb{E}_{\boldsymbol{\eta}}\left[\frac{|\nabla^{\top}_{\mathbf{x}}f(\mathbf{x}+\boldsymbol{\delta};\boldsymbol{\theta})(\boldsymbol{\delta}-\boldsymbol{\eta})|}{\|\boldsymbol{\delta}-\boldsymbol{\eta}\|_2}\right]\\[3pt]
    & &\leq&\ \ \mathbb{E}_{\boldsymbol{\eta}}\left[\frac{\|\nabla_{\mathbf{x}}f(\mathbf{x}+\boldsymbol{\delta};\boldsymbol{\theta})\|_2\|\boldsymbol{\delta}-\boldsymbol{\eta}\|_2}{\|\boldsymbol{\delta}-\boldsymbol{\eta}\|_2}\right]\\[5pt]
    & &\leq&\ \  \|\nabla_{\mathbf{x}}f(\mathbf{x}+\boldsymbol{\delta};\boldsymbol{\theta})\|_2\leq\underset{\mathbf{x}}{\textbf{max}} \|\nabla_{\mathbf{x}}f(\mathbf{x};\boldsymbol{\theta})\|_2.
    \end{aligned}
\end{equation}
The first inequality holds as the score function $f(\cdot,\cdot)$ is a convex function \textit{w.r.t} $\mathbf{x}$ and the second one holds by the H\"{o}lder inequality. It means that the proposed metric is bounded by the gradient of the adversarial perturbation $(\mathbf{x}+\boldsymbol{\delta}, \mathbf{y})$. Then it could generate the parsimonious effect on the local Lipschitzness for any $(\mathbf{x},\mathbf{y})\sim\mathcal{D}$. As a consequence, the proposed regularization could produce a more robust model than the existing adversarial training methods.

\section{More Results of Different Data Augmentation Methods}
\label{appendix:augmentation}
We adopt the PGD-10, PGD-20, PGD-50, C\&W and AA to evaluate the FGSM-BR with different data augmentation methods. The result is shown in Table~\ref{table:cifar10_augmentation}. It ii clear that using Cutout, Mixup, CutMix and AutoAugment can improve model robustness. FGSM-BR combined with Cutout achieves the best robustness performance in all attack scenarios. Specifically, under the strong AA attack, Cutout improves the performance by about 1.5\%. Moreover, Cutout also achieves comparable clean accuracy on the clean images to the vanilla FAT (FGSM-BR).

\section{Experiments with a cyclic learning rate strategy}
\label{appendix:cyclic}
All experiments are implemented by using a multi-step learning rate strategy in the manuscript. The comparative experiments are also implemented by using a cyclic learning rate strategy on CIFAR-10. Following the training settings (\cite{wong2020fast, jia2022prior}, the maximum learning rate of FGSM-GA~\cite{andriushchenko2020understanding} and FGSM-CKPT~\cite{kim2021understanding} is set to 0.3. The maximum learning rate of other FAT methods is set to 0.2. The results are shown in Table~\ref{table:cifar10_cyclic}. 
It can be observed that compared with PGD-AT, the proposed FGSM-LAW  achieves better model robustness performance under all adversarial attack scenarios and require less training cost. And compared with previous FAT methods, the proposed FGSM-LAW can achieve the best adversarial robustness under
all adversarial attack scenarios on the best and last checkpoint. In terms of the training cost, 
we observe similar phenomenons as the models trained with the multi-step learning rate strategy.

\begin{table}[t]
\centering
\caption{ Test robustness (\%) on the CIFAR-10 database using ResNet18 with equipped with Lipschitz regularization with different hyper-parameter $\lambda$ . Number in bold indicates the best. 
% Number in bold indicates the best of the fast AT methods. 
 }
\label{table:HP_regular}
\scalebox{0.92}{
\begin{tabular}{@{}c|c|c|c|c|c|c|c@{}}
\toprule
 Hyper-Parameter & Clean          & PGD-10         & PGD-20         & PGD-50         & C\&W           & AA             & Time \\ \midrule
Baseline    & \textbf{86.82} & 46.62  & 44.76  & 44.23  & 45.89 & 42.37  & 1 $\times$    \\ \midrule \midrule
$\lambda=8$      & 84.34 & 54.09          & 53.21          & 52.88          & 49.28          & 46.57          & 1.4 $\times$ \\ \midrule
$\lambda=10$     & 84.04          & 84.04          & 54.31          & 53.03          & 49.83          & 47.08          & 1.4 $\times$ \\ \midrule
$\lambda=12$     & 83.35          & 53.94          & 54.03          & 53.66          & 50.05          & 47.38          & 1.4 $\times$ \\ \midrule
$\lambda=14$    & 82.97          & \textbf{55.49} & \textbf{54.58} & \textbf{54.29} & \textbf{50.41} & \textbf{48.05} & 1.4 $\times$ \\ \midrule
$\lambda=16$     & 83.49          & 54.86          & 53.99          & 53.62          & 49.53          & 47.11          & 1.4 $\times$  \\ \midrule
$\lambda=18$     & 82.74          & 55.2           & 54.35          & 54.27          & 50.17          & 47.58          & 1.4 $\times$  \\ \bottomrule
\end{tabular}
}
\end{table}

\begin{table}[t]
\centering
\caption{ Test robustness (\%) on the CIFAR-10 database using ResNet18 equipped with auto weight averaging with diffrerent hyper-parameters $\Delta$. Number in bold indicates the best. 
% Number in bold indicates the best of the fast AT methods. 
 }
\label{table:HP_WA}
\scalebox{0.92}{
\begin{tabular}{@{}c|c|c|c|c|c|c|c@{}}
\toprule
Hyper-Parameter & Clean & PGD-10         & PGD-20        & PGD-50         & C\&W           & AA             & Time \\ \midrule
Baseline    & \textbf{86.82} & 46.62  & 44.76  & 44.23  & 45.89 & 42.37  & 1 $\times$    \\ \midrule \midrule
$\Delta=0.6$    & 79.98 & 51.47 & \textbf{50.7} & \textbf{50.53} & 48.53          & 46.08          & 1 $\times$   \\ \midrule
$\Delta=0.65$   & 80.92 & \textbf{51.69}          & 50.9          & 49.73          & 49.15          & 46.18          & 1 $\times$   \\ \midrule
$\Delta=0.7$    & 81.82 & 50.94          & 50.11         & 49.85          & 49.21          & 46.22          & 1 $\times$    \\ \midrule
$\Delta=0.75$   & 83.62 & 51.26          & 50.21         & 49.9           & \textbf{49.42} & \textbf{46.53} & 1 $\times$   \\ \midrule
$\Delta=0.8$    & 85.76 & 48.9           & 47.35         & 46.89          & 47.59          & 44.33          & 1 $\times$   \\ \midrule
$\Delta=0.85$   & 86.7  & 47.83          & 46.04         & 45.68          & 46.84          & 43.47          & 1 $\times$   \\ \bottomrule
\end{tabular}
}
\end{table}

\section{Detailed hyper-parameter settings}
\label{appendix:hyper-parameter}
There are two hyper-parameters in the proposed FGSM-LAW, \emph{i.e,}
the hyper-parameter of the Lipschitz regularization $\lambda$ and the hyper-parameter of the auto weight averaging $\Delta$. Using ResNet18 on CIFAR-10, we adopt the FGSM-BR combined with Lipschitz regularization and auto weight averaging to determine the optimal hyper-parameters, respectively. As for the hyper-parameter $\lambda$, the results are shown in Table~\ref{table:HP_regular}. It can be observed that when $\lambda=14$, the proposed Lipschitz regularization can achieve the best model robustness  under all attack scenarios. In detail, under AA attack, the proposed Lipschitz regularization achieves an accuracy of about 48\%. Hence, the hyper-parameter $\lambda$ of the proposed Lipschitz regularization is set to 14. As for the hyper-parameter $\Delta$, the results are shown in Table~\ref{table:HP_WA}. It can be observed that when $\Delta =0.75$, the proposed auto weight averaging can achieve the best model robustness  under C\&W and AA attack scenarios. Considering the clean accuracy on clean samples, the hyper-parameter $\Delta$ of the proposed auto weight averaging is set to 0.75.

\begin{table}[t]
\centering
\caption{ Test robustness (\%) on the Tiny ImageNet database using PreActResNet18 with different adversarial training methods. Number in bold indicates the best. 
% Number in bold indicates the best of the fast AT methods. 
}
\label{table:Tiny_ImageNet}
\scalebox{0.82}{
\begin{tabular}{@{}c|c|c|c|c|c|c|c@{}}
\toprule
Method       & \begin{tabular}[c]{@{}c@{}}Clean\\ Best/Last\end{tabular} & \begin{tabular}[c]{@{}c@{}}PGD-10\\ Best/Last\end{tabular} & \begin{tabular}[c]{@{}c@{}}PGD-20\\ Best/Last\end{tabular} & \begin{tabular}[c]{@{}c@{}}PGD-50\\ Best/Last\end{tabular} & \begin{tabular}[c]{@{}c@{}}C\&W\\ Best/Last\end{tabular} & \begin{tabular}[c]{@{}c@{}}AA\\ Best/Last\end{tabular} & Time \\ \midrule
PGD-AT       & 43.6/45.28                                                  & 20.2/16.12                                                   & 19.9/15.6                                                    & 19.86/15.4                                                   & 17.5/14.28                                                 & 16.0/12.84                                               & 5.2$\times$   \\ \midrule \midrule
FGSM-RS      & 44.98/45.18                                                 & 17.72/0.00                                                   & 17.46/0.00                                                   & 17.36/0.00                                                   & 15.84/0.00                                                 & 14.08/0.00                                               & 1 $\times$    \\ \midrule
FGSM-PGI     & 43.32/45.88                                                 & 23.8/22.02                                                   & 23.4/21.7                                                    & 23.38/21.6                                                    & 19.28/17.44                                                & \textbf{17.56}/15.50                                              & 1.4 $\times$   \\ \midrule
FGSM-CKPT    & \textbf{49.98/49.98}                                        & 9.20/9.20                                                    & 9.20/9.20                                                    & 8.68/8.68                                                    & 9.24/9.24                                                  & 8.10/8.10                                                & 1.5 $\times$   \\ \midrule
FGSM-SDI     & 46.46/47.64                                                 & 23.22/19.84                                                  & 22.84/19.36                                                  & 22.76/19.16                                                  & 18.54/16.02                                                & 17.0/14.10                                               & 1.6 $\times$   \\ \midrule
NuAT         & 42.9/42.42                                                  & 15.12/13.78                                                  & 14.6/13.34                                                   & 14.44/13.2                                                   & 12.02/11.32                                                & 10.28/9.56                                               & 2.0 $\times$   \\ \midrule
GAT          & 42.16/41.84                                                 & 15.02/14.44                                                  & 14.5/13.98                                                   & 14.44/13.8                                                   & 11.78/11.48                                                & 10.26/9.74                                               & 2.0 $\times$   \\ \midrule
FGSM-GA      & 43.44/43.44                                                 & 18.86/18.86                                                  & 18.44/18.44                                                  & 18.36/18.36                                                  & 16.2/16.2                                                  & 14.28/14.28                                              & 3.5 $\times$   \\ \midrule
Free-AT (m=8) & 38.9/40.06                                                  & 11.62/8.84                                                   & 11.24/8.32                                                   & 11.02/8.2                                                    & 11.00/8.08                                                 & 9.28/7.34                                                & 4.2 $\times$   \\ \midrule
FGSM-LAW (ours)    & 47.74/47.74                                                 & \textbf{24.45/24.45}                                         & \textbf{24.09/24.09}                                         & \textbf{24.06/24.06}                                         & \textbf{18.65/18.65}                                       & 16.43/\textbf{16.43}                                     & 1.4 $\times$ \\ \bottomrule
\end{tabular}
}
\end{table}
\input{table/ImageNet}
\section{Experiments with WideResNet34-10 as the backbone}
\label{appendix:WideResNet}
We adopt a larger architecture (WideResNet34-10) as the backbone to conduct comparative experiments on CIFAR-10. 
The results are shown in Table~\ref{table:cifar10_wide}. It can be observed that compared with PGD-AT, the proposed FGSM-LAW achieves better model robustness. Particularly, under AA attack, PGD-AT achieves an
accuracy of about 51\%, while the proposed FGSM-LAW achieves an accuracy of about 52\%. Compared with previous FAT methods, the proposed method achieves the best robustness performance under all attack scenarios. In terms of the training cost, 
we observe similar phenomenons as ResNet18 used as the backbone. 

\section{Experiments on Tiny ImageNet and ImageNet}
\label{appendix:ImageNet}
\par \textbf{Results on Tiny ImageNet}
Compared with CIFAR-10 and CIFAR-100, Tiny ImageNet is a larger database that covers more classes. It is hard to obtain robustness on Tiny ImageNet
As for Tiny ImageNet, following~\cite{jia2022boosting,jia2022prior}, we adopt PreActResNet18 as the backbone to
conduct experiments. The results are shown in Table~\ref{table:Tiny_ImageNet}.  It can be observed that compared with PGD-AT, the proposed FGSM-LAW achieves better model robustness and requires less training time. And compared with previous FAT methods, the proposed method achieves the best model robustness under most attack scenarios and comparable robustness to the advanced FAT method (FGSM-PGI) under AA attack. However, compared with FGSM-PDI, the proposed FGSM-LAW achieves better model robustness under all attack scenarios without extra data memory. In terms of the training cost, we can observe similar phenomenons as the model trained on CIFAR-10 and CIFAR-100. 

% \section{Description of the databases}
% \label{appendix:databases}
% CIFAR-10, CIFAR-100, Tiny ImageNet and ImageNet databases are widely used to evaluate the model robustness. 
% 50,000 training images and 10,000 test images make up of the CIFAR-10 dataset. It covers covers 10 classes of
% images with $32 \times 32$. 

\par \textbf{Results on ImageNet}
Following the training settings ~\citep{shafahi2019adversarial,wong2020fast}, we adopt ResNet50 as the backbone to conduct comparative experiments. The maximum perturbation strength $\epsilon$ is set to 8/255. We compare the proposed FGSM-LAW with PGD-AT \citep{madry2017towards}, Free-AT \citep{shafahi2019adversarial} and FGSM-RS \citep{wong2020fast}. 
% Combined with their leaderboard results~\footnote{https://github.com/alibaba/easyrobust}, 
The results are shown in Table~\ref{table:ImageNet}. Compared with PGD-AT, our FGSM-LAW achieves higher clean accuracy and comparable robustness under AA attack. Compared with Free-AT and FGSM-RS, the proposed FGSM-LAW achieves the best clean and robust accuracy.
